# Supplementary material for: Probing Metal-Molecule Contact at the Atomic Scale via Conductance Jump
Source: arXiv:2109.04078 ancillary file (2021-09-09)
Supplement: Supplementary file 1 [file Supplementary_Information.pdf]

# **Probing Metal-Molecule Contact at the Atomic Scale via Conductance Jump**

Biswajit Pabi, Debayan Mondal, Priya Mahadevan\*, and Atindra Nath Pal\*

Department of Condensed Matter Physics and Material Science, S. N. Bose National Center for Basic Science, Sector III, Block JD, Salt Lake, Kolkata - 700106

Email: atin@bose.res.in, priya@bose.res.in

## **Supplementary Information**

### **Contents**

**Supplementary Note 1: Electronic circuit for conductance measurements**

**Supplementary Note 2: 2D conductance density plot of pull traces**

**Supplementary Note 3: Plateau length histogram**

**Supplementary Note 4: Jump to contact detection**

**Supplementary Note 5: Correlation analysis**

**Supplementary Note 6: Bar diagram details**

**Supplementary Note 7: Conditional analysis for 4, 4'-BPY (pull traces)**

**Supplementary Note 8: Details of theoretical calculations**

**Supplementary Note 9: Density of states of 4, 4'-BPY on Au surface**

### Supplementary Note 1: Electronic circuit for conductance measurements

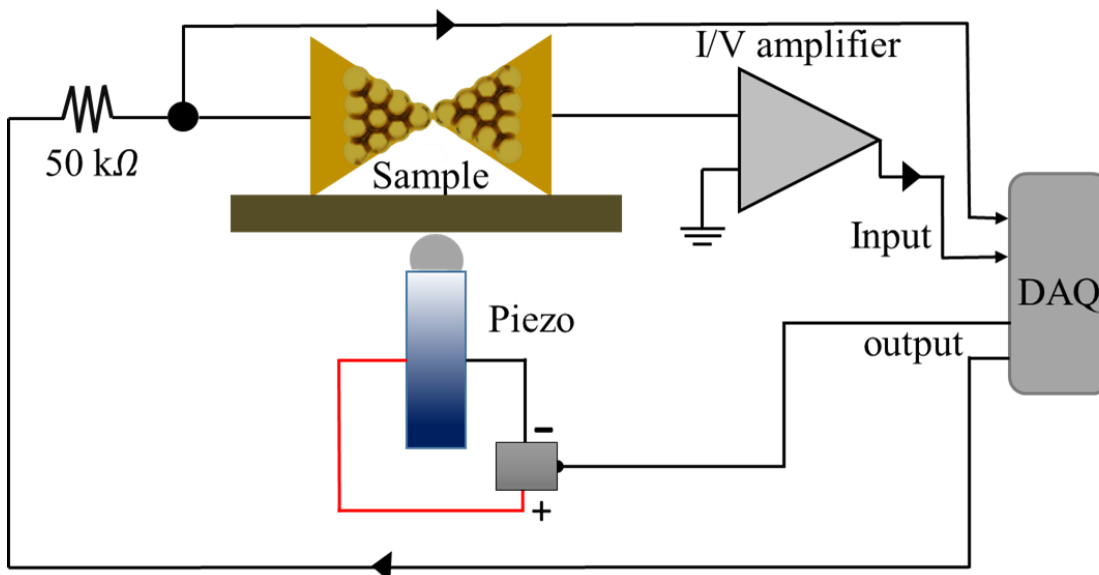

**Figure S1.** Schematic of the electronic circuit used for dc conductance measurements.

The electrical circuit mentioned above was used to measure the electrical conductance of single molecular junction for our experiments. To record conductance-distance traces, a triangular waveform was applied on the piezoelectric element to break and make the junctions consecutively. For measuring conductance, a dc bias was applied from the output channel of a 24 bit DAQ card (PCI 4461, NI Instruments) and the current was amplified by a current to voltage preamplifier (SP 983, electronics lab, University of Basel) and measured by the input channel of the DAQ card. As the conductance of the junctions varying rapidly while breaking the wire, it is a challenge to measure the conductance of the junction effectively by keeping the preamplifier gain constant. A 50 k $\Omega$  resistance was used in series to circumvent this problem and it helps to limit the current while the junction conductance is high<sup>1</sup>. By measuring the current through the circuit, along with the voltage drop across the junction, one can measure the conductance of the junction. Voltage drop across the junction can be calculated using the following formula,

$$V_{\text{bias}} = V_{50} + V_{\text{sample}}$$

$$V_{\text{sample}} = V_{\text{bias}} - V_{50}$$

$$G_{\text{sample}} = I/V_{\text{sample}} = I/ (V_{\text{bias}} - V_{50})$$

( $V_{\text{bias}}$ =bias voltage,  $V_{50}$ =voltage drop across the 50 k $\Omega$  resistance,  $V_{\text{sample}}$ =voltage drop across the sample,  $I$ =current)

## Supplementary Note 2: 2D conductance density plot for pull traces

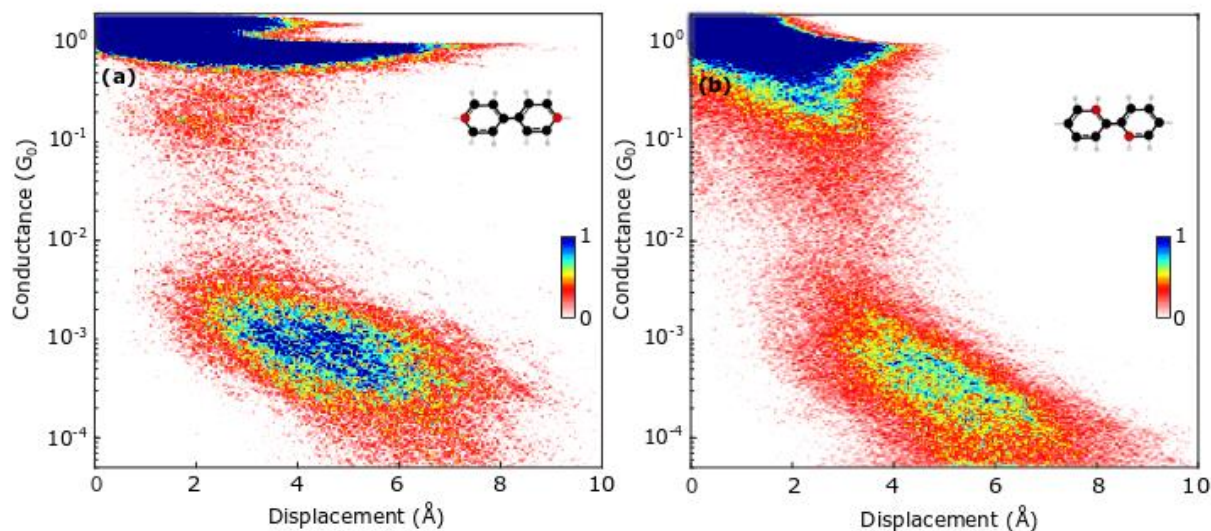

**Figure S2.** 2D Conductance-displacement density plot for (a) 4, 4'-BPY and (a) 2, 2'-BPY for pull traces and is constructed from the same 5000 & 8000 traces as used in the conductance histogram of Figure 3c & figure 3e of the main text, using 50bins per decade.

## Supplementary Note 3: Plateau length histogram

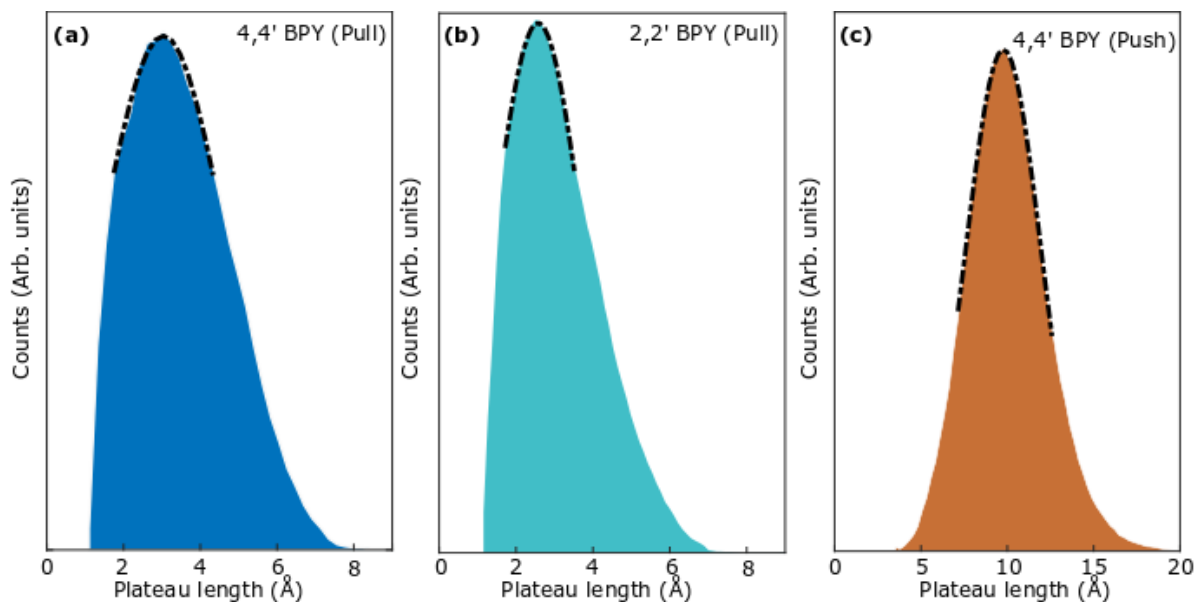

**Figure S3.** Plateau length histogram constructed by analyzing 3352 pull traces (a), 5000 push traces (c) of 4, 4'-BPY molecular junction and 3778 pull traces (b) of 2, 2'-BPY molecular junction. Black dash-dot line depict a fit to a Gaussian distribution, yielding an average plateau length of  $3.03 \pm 0.02 \text{ \AA}$  (pull plateaus of 4, 4'-BPY),  $2.57 \pm 0.01 \text{ \AA}$  (pull plateaus of 2, 2'-BPY),

$9.77 \pm 0.01 \text{ \AA}$  ( push plateaus of 4, 4'-BPY). Similar values of  $2.1 \text{ \AA}$  and  $3.2 \text{ \AA}$  were found for 2,2'-BPY and 4,4'-BPY respectively from DFT calculations carried out for several elongations and examining the eigenfunctions to see where the coupling between the molecule and the electrode went to zero.

#### Supplementary Note 4: Jump to contact detection

To detect the jump in the conductance traces, the following algorithm was developed. Each conductance trace consists of equally spaced piezo bias (which translates to displacement) and corresponding conductance values. We calculate the ratio between the consecutive conductance values. We define a threshold value for jump ( $\Delta G_{\text{jump}}$ ) and the jump is identified whenever the ratio,  $G_n/G_{n+1} > \Delta G_{\text{jump}}$ . This is pictorially presented in SI Figure S4a. Figure S4b shows three push traces with two characteristic jumps, detected using the scheme mentioned above. The first jump corresponds to the one from the noise background to the onset of molecular junction formation ( $\sim 10^{-3}G_0$ ), and another jump to a conductance above  $\sim 0.5G_0$  from  $G \sim 0.1G_0$ , depicting the formation of metallic contact.

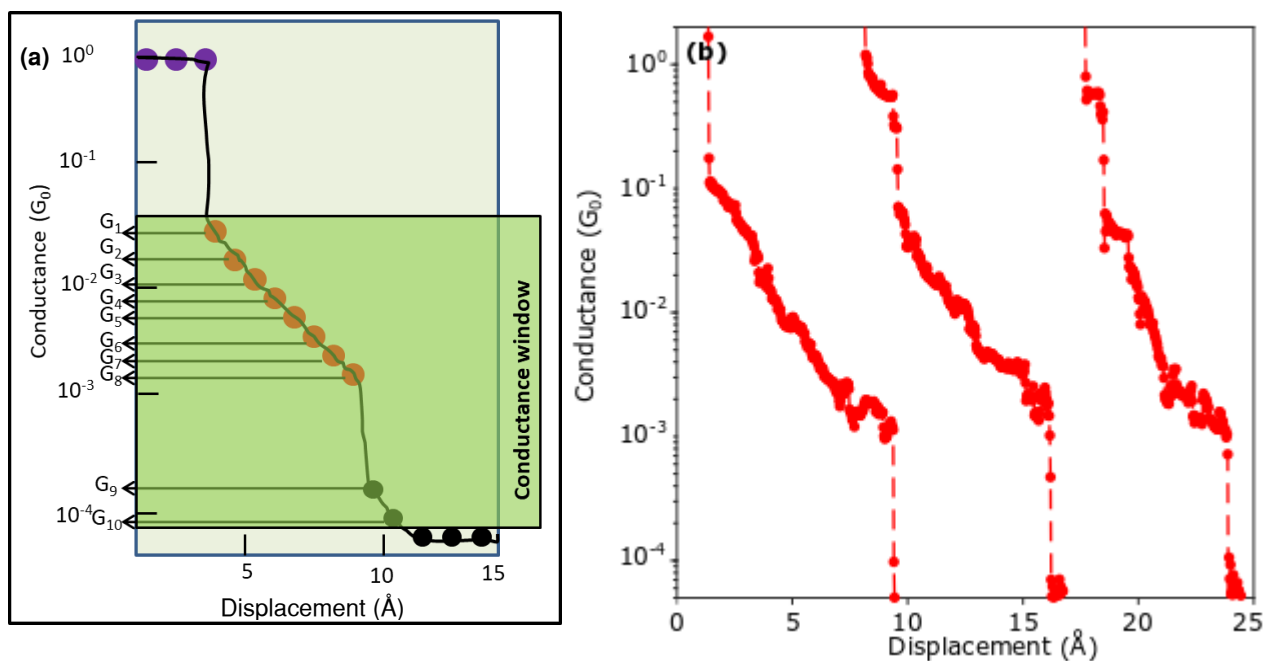

**Figure S4.** (a) Schematic of a conductance trace, explaining the jump detection algorithm. (b) Experimental conductance traces (push) for 4, 4'-BPY for which molecular junction is formed via jump from the noise background or tunneling.

#### Supplementary Note 5: Correlation analysis

For a typical break junction experiment, conductance of the junction is measured as a function of electrode separation during junction opening and closing process. This breaking and making processes are repeated several times to look into the junction's property statistically and one complete measurement cycle is called "*conductance trace*". Conductance histogram is then constructed by compiling these conductance traces and a peak in the histogram corresponds to the conductance of the most frequently occurring junction configuration or the most probable junction configuration. Conductance histogram, however, can only provide us the conductance of the most probable junction and to overcome this limitation several attempts were proposed like plateaus length analysis<sup>2, 3</sup> to validate atomic chain formation, 2D conductance displacement histogram<sup>4</sup> to check the evolution of conductance upon stretching, correlation analysis<sup>5</sup> to understand the various junction evolution trajectories and so on.

Correlation analysis, introduced by the Halbeter and coworkers<sup>5</sup>, is an extremely useful tool to detect the several features of junction formation and evolution, which cannot be accessible using conventional conductance histogram. To obtain the statistical relation between different junction configurations having its characteristics conductance value, correlation parameter can be defined as,

$$C_{m,n} = \frac{\langle \delta N_m(r) * \delta N_n(r) \rangle_r}{\sqrt{\langle [\delta N_m(r)]^2 \rangle_r * \langle [\delta N_n(r)]^2 \rangle_r}}$$

Where  $N_m(r)$  and  $N_n(r)$  are the number of data points in the  $m^{\text{th}}$  and  $n^{\text{th}}$  bin of the given trace  $r$ .  $\delta N_{m/n}(r) = N_{m/n}(r) - \langle N_{m/n}(r) \rangle$  is the deviation from the mean value. Let's discuss the value of  $C_{m,n}$  along with its physical significance-

- (a)  $C_{m,n} = 0$ ; Configurations are statistically independent.
- (b)  $C_{m,n} \neq 0$ ; Configurations are statistically dependent and type of dependency is determined by the sign of the function. Positive values of  $C_{m,n}$  leads to the positive correlation and for these cases configurations either appear or disappear together. Negative value of the function indicate negative correlation and more than average counts in one configuration is supported by the less than average counts in another configuration. It may also be the situation that formation of one configuration resists the formation of other.

Similar function can also be used to understand the cross-correlation between the opening and its corresponding closing traces<sup>6</sup>. This may help us to understand the post-rupture evolution of the molecular junction and one may conclude regarding the situation of junction after breaking (whether molecule attached to one of the electrode or diffuse away from the junction). The function can slightly be modified as,

$$C_{m,n} = \frac{\langle \delta N_m(r) * \delta N'_n(r) \rangle_r}{\sqrt{\langle [\delta N_m(r)]^2 \rangle_r * \langle [\delta N'_n(r)]^2 \rangle_r}}$$

Here  $r$  denotes the entire opening-closing cycle,  $N_m(r)$  is the number of data points in the  $m^{\text{th}}$  bin of the opening trace, whereas  $N'_n(r)$  is the number of data points in the  $n^{\text{th}}$  bin of the closing traces. In contrast to the former function, diagonal of the opening-closing cross-correlation function is not unity. This function was used in reference 7 to indicate the structure-memory effects<sup>7</sup> in atomic size contacts and molecular junctions. To check the post rupture evolution of our system under study, we are using this same function for which number of data points in each bin is calculated by logarithmic binning.

#### Supplementary Note 6: Bar diagram details

| Data set | Total number of traces ( $N_{\text{Total}}$ ) | Total number of traces ( $N_{\text{jump}}$ ) with jump in <i>push</i> (% inside bracket) | Total number of traces ( $N_{\text{mol}}$ ) having both jump in <i>push</i> and molecule in <i>pull</i> (% inside bracket) | $N_{\text{mol}}/N_{\text{jump}}$ (%) |
|----------|-----------------------------------------------|------------------------------------------------------------------------------------------|----------------------------------------------------------------------------------------------------------------------------|--------------------------------------|
| 1        | 5000                                          | 3750 (75.00)                                                                             | 3236 (64.72)                                                                                                               | 86.29                                |
| 2        | 2500                                          | 1765 (70.60)                                                                             | 1398 (55.92)                                                                                                               | 79.20                                |
| 3        | 3500                                          | 2510 (71.71)                                                                             | 2066 (59.02)                                                                                                               | 82.31                                |
| 4        | 3200                                          | 2155 (67.34 )                                                                            | 1770 (55.31)                                                                                                               | 82.13                                |
| 5        | 5000                                          | 2991 (59.82)                                                                             | 2232 (44.64)                                                                                                               | 74.62                                |
| 6        | 10000                                         | 6946 (69.46)                                                                             | 5470 (54.70)                                                                                                               | 78.75                                |
| 7        | 9000                                          | 6469 (71.87)                                                                             | 5418 (60.2)                                                                                                                | 83.75                                |
| 8        | 10000                                         | 7396 (73.96)                                                                             | 6020 (60.2)                                                                                                                | 81.39                                |

#### Supplementary Note 7: Conditional histogram analysis for 4, 4'-BPY molecular junction (pull traces)

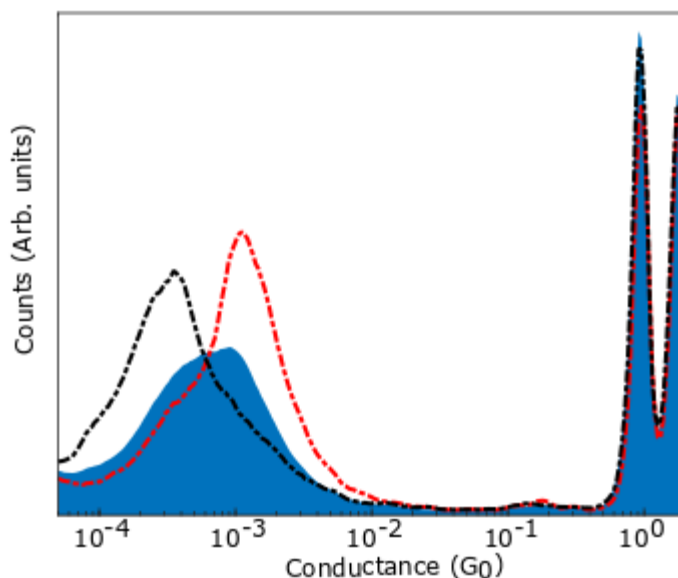

**Figure S5.** 1D logarithmic conductance histogram of 4, 4'-BPY single molecular junction where blue area plot is constructed from the traces having molecule. Red dash line & black dash line correspond to the histogram for which molecular plateaus lie in the high conductance regime & low conductance regime respectively and confirmed from the negative correlation<sup>8, 5</sup>.

### **Supplementary Note 8: Details of theoretical calculations**

In order to model the experiments, we use density functional theory based ab-initio electronic structure calculations using the generalised gradient approximation (Perdew Burke-Ernzerhof)<sup>9</sup> for the exchange correlational functional as implemented within Vienna ab initio simulation package (VASP)<sup>10-13</sup>. In some instances, we have also carried out molecular dynamics (MD) simulation<sup>14</sup> which provides us with some insights on how the molecule breaks.

The ab-initio MD simulations were carried out at room temperature (300K) for several molecular junctions formed by 4, 4'-BPY and 2, 2'-BPY molecules with gold electrodes. The optimized structure of a gold slab–molecule–gold slab is used to construct the junction atomic geometry, where 8 layers were used to construct the slab. The slabs are separated by a vacuum of 15 Å. The electrodes are pulled apart in steps of 0.1 Å. The entire system is relaxed at every step by taking 200 MD steps of 0.5 fs. The whole system is kept at the desired target temperature in NVT canonical ensemble using a Nosé-Hoover thermostat<sup>15-17</sup>.

We also included dispersion-corrections using the DFT-D2 method due to Grimme<sup>18-21</sup>. Van der Waals interactions are believed to provide a more accurate description of the long-range interactions between atoms and molecules in vacuum slabs. The k-space sampling is restricted to the  $\Gamma$  point only<sup>22</sup>. We have also used a plane-wave cut-off of 500 eV for the plane waves included in the basis.

Zero temperature relaxations were also done for certain geometries of the molecule-Au structures as well as Au only structures. These were subject to elongation and the energy as a function of strain was evaluated. The energy convergence was set at  $10^{-5}$  eV, while the structural relaxations were carried out till forces were less than  $10^{-3}$  eV/atom. Density of states were calculated using spheres of radii 2.84 Å and 1.40 Å for Au and N respectively and have been broadened by Gaussians with full width at half maxima of 0.01 eV.

### **Supplementary Note 9: Density of states of 4, 4'-BPY on Au surface**

Density of states have been calculated for the optimized structure where 4, 4'-BPY is placed vertically on gold surface. The charge density mentioned in the main manuscript (Figure 5a (inset)) have been calculated for the state 'A' in the graph (S6).

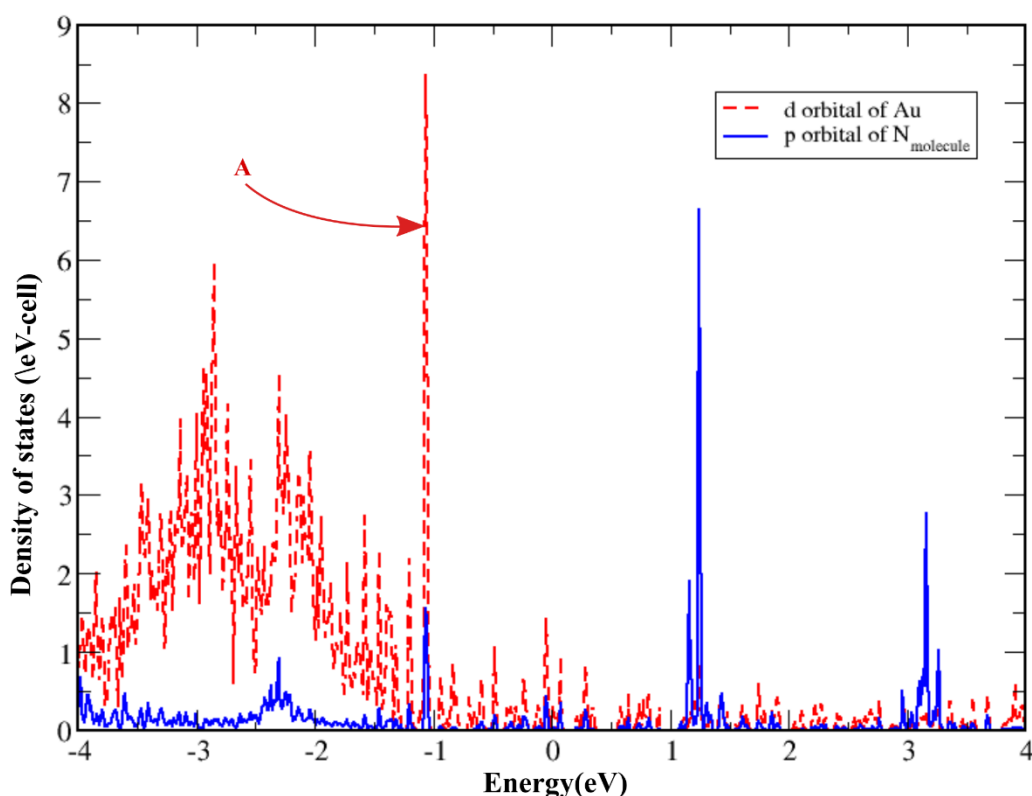

**Figure S6.** The calculated Au d (red) and N (4, 4'-BPY) p (blue) contributions to the broadened density of states.

#### Reference:

1. Kamenetska, M. Single molecule junction conductance and binding geometry, *Phd. thesis*, Columbia University, New York (2012).
2. Yanson, A. I., Rubio Bollinger, G., Van Den Brom, H. E., Agraït, N. & Van Ruitenbeek, J. M. Formation and manipulation of a metallic wire of single gold atoms. *Nature* **395**, 783–785 (1998).
3. Untiedt, C. *et al.* Calibration of the length of a chain of single gold atoms. *Phys. Rev. B - Condens. Matter Mater. Phys.* **66**, 854181–854186 (2002).
4. Kamenetska, M. *et al.* Formation and evolution of single-molecule junctions. *Phys. Rev. Lett.* **102**, 2–5 (2009).
5. Makk, P. *et al.* Correlation analysis of atomic and single-molecule junction conductance. *ACS Nano* **6**, 3411–3423 (2012).
6. Balogh, Z. *et al.* Precursor configurations and post-rupture evolution of Ag-CO-Ag single-molecule junctions. *Nanoscale* **6**, 14784–14791 (2014).
7. Magyarkuti, A. *et al.* Temporal correlations and structural memory effects in break

- junction measurements. *J. Chem. Phys.* **146**, (2017).
8. Quek, S. Y. *et al.* Mechanically controlled binary conductance switching of a single-molecule junction. *Nat. Nanotechnol.* **4**, 230–234 (2009).
  9. Perdew, J. P., Burke, K. & Ernzerhof, M. Generalized Gradient Approximation Made Simple. *Phys. Rev. Lett.* **77**, 3865–3868 (1996).
  10. Kresse, G. & Furthmüller, J. Efficient iterative schemes for ab initio total-energy calculations using a plane-wave basis set. *Phys. Rev. B* **54**, 11169–11186 (1996).
  11. Kresse, G. & Hafner, J. Ab initio molecular dynamics for liquid metals. *Phys. Rev. B* **47**, 558–561 (1993).
  12. Kresse, G. & Furthmüller, J. Efficiency of ab-initio total energy calculations for metals and semiconductors using a plane-wave basis set. *Comput. Mater. Sci.* **6**, 15–50 (1996).
  13. Kresse, G. & Hafner, J. Ab initio molecular-dynamics simulation of the liquid-metal--amorphous-semiconductor transition in germanium. *Phys. Rev. B* **49**, 14251–14269 (1994).
  14. Frenkel, D. & Smit, B. *Understanding Molecular Simulation: From Algorithms to Applications*. (Academic Press, Inc., 1996).
  15. Nosé, S. A unified formulation of the constant temperature molecular dynamics methods. *J. Chem. Phys.* **81**, 511–519 (1984).
  16. Shuichi, N. Constant Temperature Molecular Dynamics Methods. *Prog. Theor. Phys. Suppl.* **103**, 1–46 (1991).
  17. Hoover, W. G. Canonical dynamics: Equilibrium phase-space distributions. *Phys. Rev. A* **31**, 1695–1697 (1985).
  18. Grimme, S. Semiempirical GGA-type density functional constructed with a long-range dispersion correction. *J. Comput. Chem.* **27**, 1787–1799 (2006).
  19. Egger, D. A. & Kronik, L. Role of Dispersive Interactions in Determining Structural Properties of Organic–Inorganic Halide Perovskites: Insights from First-Principles Calculations. *J. Phys. Chem. Lett.* **5**, 2728–2733 (2014).
  20. Wang, Y. *et al.* Density functional theory analysis of structural and electronic properties of orthorhombic perovskite CH<sub>3</sub>NH<sub>3</sub>PbI<sub>3</sub>. *Phys. Chem. Chem. Phys.* **16**, 1424–1429 (2014).
  21. Lee, K., Murray, É. D., Kong, L., Lundqvist, B. I. & Langreth, D. C. Higher-accuracy van der Waals density functional. *Phys. Rev. B* **82**, 81101 (2010).
  22. Monkhorst, H. J. & Pack, J. D. Special points for Brillouin-zone integrations. *Phys. Rev. B* **13**, 5188–5192 (1976).
